# Supplementary material for: Returning CP-Observables to The Frames They Belong
Source: arXiv:2308.00027 source file (2023-07-31)

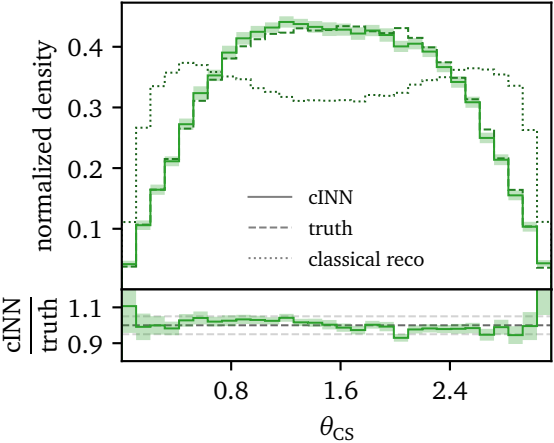

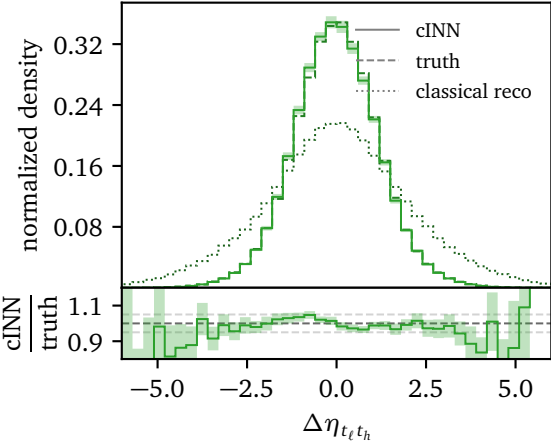

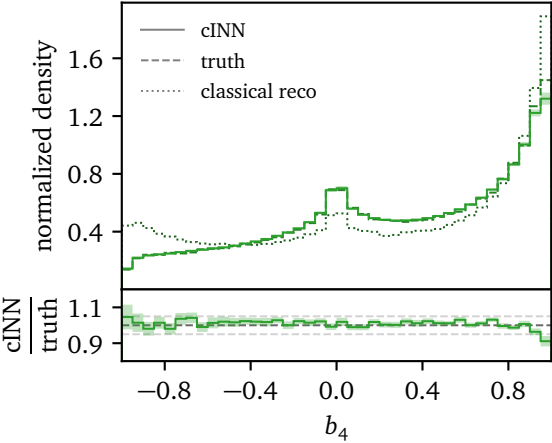

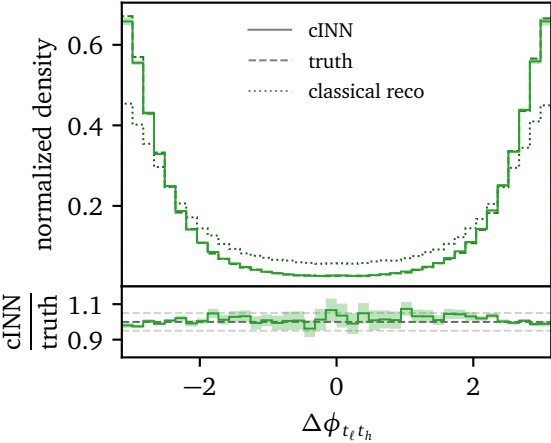

Supplement: Supplementary file 1 [file model_precision_sm.pdf]
