# Supplementary material for: Returning CP-Observables to The Frames They Belong
Source: arXiv:2308.00027 source file (2023-07-31)

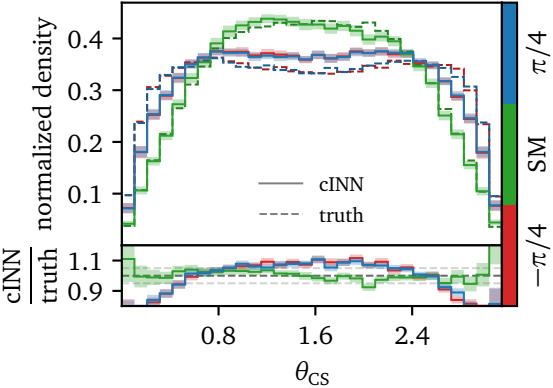

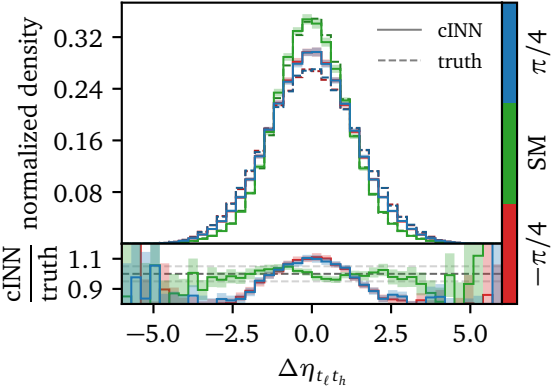

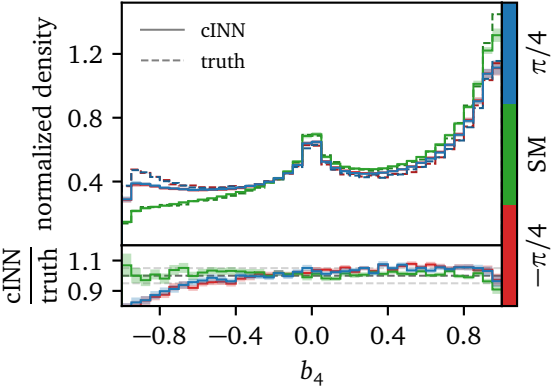

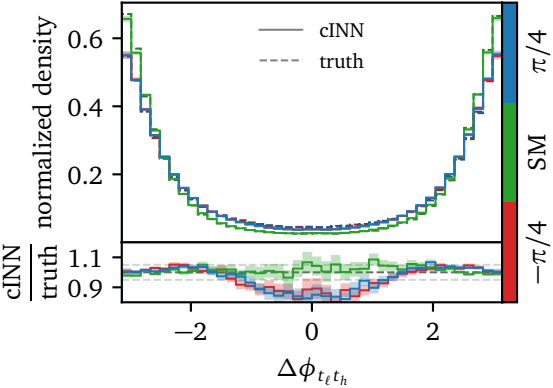

Supplement: Supplementary file 2 [file unfold_hypotheses_under_sm.pdf]
