# Supplementary material for: Returning CP-Observables to The Frames They Belong
Source: arXiv:2308.00027 source file (2023-07-31)

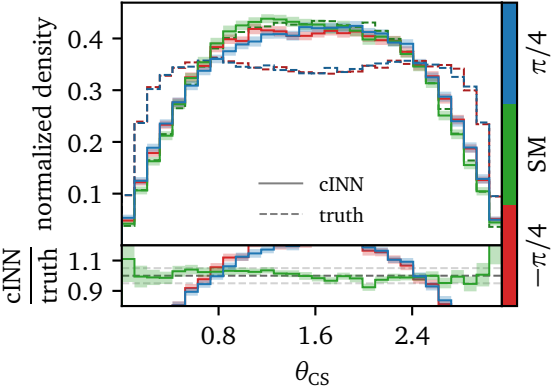

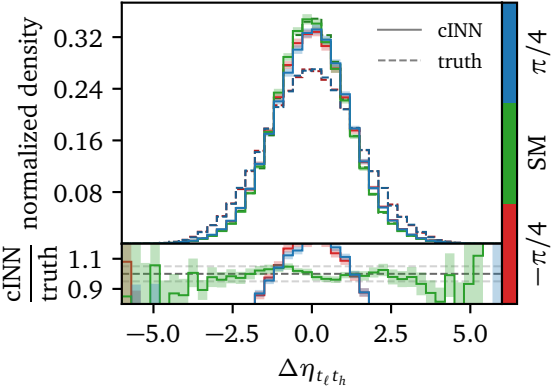

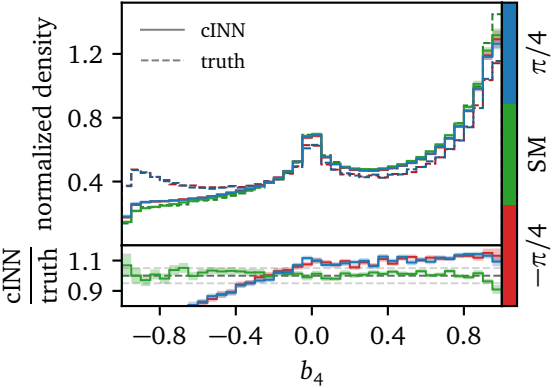

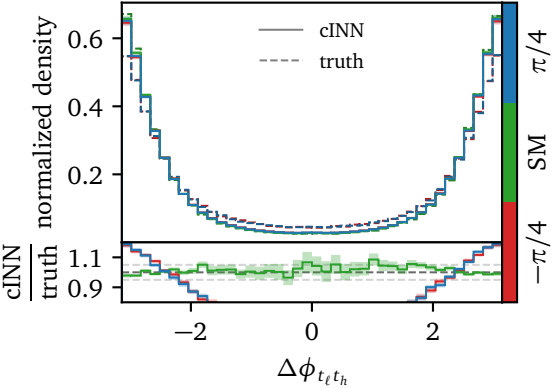

Supplement: Supplementary file 3 [file unfold_sm_full.pdf]
